# Supplementary material for: Semi-Supervised Laplace Learning on Stiefel Manifolds
Source: arXiv:2308.00142 source file (2024-08-14)
Supplement: Supplementary file 2 [file appendix_backup_backup.tex]

\textbf{Overview of supplemental material.}
In Section~\ref{sec:additionalresults}, we provide additional numerical evidence for the efficacy of our framework compared to a larger variety of methods for graph-based semi-supervised learning. We also explore the effect of the label rate at a higher resolution and compare our proposed SSM algorithm to existing open-source implementations of classic algorithms for Riemannian optimization. 
%In Section~\ref{sec:sqp}, we describe the proposed SSM algorithm in detail. We introduce the algorithm and derive the update rule and discuss the computational cost of performing iterations of SSM. In Section~\ref{sec:cutrefinement}, we introduce the KL refinement step. 
In Section~\ref{sec:activelearning}, we discuss an alternative perspective of our active learning score. This alternative perspective is inspired by recent literature on noise-robust sampling techniques developed in the context of graph signal processing. We derive a lower-bound on the smallest eigenvalue of $L_\mathcal{U}$ and demonstrate that our score is a good proxy for this bound. This implication of this bound is that our algorithm can be interpreted a greedy algorithm for degree-weighted uncertainty sampling that is robust to any underlying noise in the data or graph construction. In Section~\ref{sec:ssmconvergence}, we provide a theoretical analysis of SSM with the goal of developing a convergence result for the algorithm. We conclude the supplemental material in Section~\ref{sec:limitations} by discussing the limitations of our work and the broader societal impact of graph-based semi-supervised learning. 

\section{Additional Results}
\label{sec:additionalresults}
Here, we provide additional numerical evidence for the efficacy of our framework, compared to a larger variety of graph-based semi-supervised learning algorithms.
%\subsection{Embeddings and barcode plots}
%
%

\subsection{Benchmarking graph-based semi-superivsed learning algorithms}
In this section, we provide extended results on our proposed methods. First, we present average accuracy scores over additional label rates on MNIST, Fashion MNIST, and CIFAR-10. 
We compare our SSM approach and alignment-based approximation presented in section \ref{sec:approx} (Procrustes-SSL) against Laplace learning \cite{zhu2003semi}, Poisson learning \cite{calder20poisson}, lazy random walks \cite{zhou2004lazy,zhou2004learning},  weighted nonlocal Laplacian (WNLL) \cite{shi2017weighted}, $p$-Laplace  learning \cite{flores2019algorithms}, and Laplacian Eigenmaps SSL (LE-SSL)\cite{Belkin2002UsingMS}. 
We restrict our comparison to methods \emph{without additional cut-based refinement} (e.g. PoissonMBO or KL), which we provide in the following table. 

We conduct additional experiments to compare Procrustes-SSL + MBO, SSM + MBO, PoissonMBO, VolumeMBO at low ($1$, $3$, $5$) and high ($4000$) label-rates. Importantly, to conduct a fair comparison, we have augmented our proposed methods with the MBO-based refinement procedure proposed in Sec 2.4 of ~\citet{calder20poisson} with the same set of parameters. This amounts to replacing the PoissonLearning step (line 3, Algorithm 2 of \citet{calder20poisson}) with either of our proposed methods (Procrustes-SSL or SSM). We show that when our method is augmented with this additional refinement step, we gain significant improvements in solution quality as well as smaller standard deviation while outperforming all MBO-based approaches. This trend notably persists through the high-label-rate regime.


Next, we evaluate the ability of our approach to retain strong predictive performance at medium and high label rates. Here, we show that Poisson Learning fails to retain superior results as compared to Laplace Learning. 
\input{tables/mnistresults.tex}
\input{tables/fmnistresults.tex}
\input{tables/CIFAR10results.tex}
\input{tables/mbo}
\input{tables/scaling.tex}

\subsection{Comparison with an open-source tool for Riemannian optimization}
\input{tables/pymanopt}
\input{figures/results.tex}
Additionally, we include a comparison between the SSM component of our framework and the general first (RG) and second-order (TR) Riemannian optimization algorithms implemented in the Pymanopt package~\cite{pymanopt}. For submanifolds of Euclidean spaces, first-order methods for constrained problems that consist of iteratively taking a tangent step in the Euclidean space followed by a projection (i.e. our projected gradient method) are functionally equivalent to Riemannian Gradient methods~\cite{absil07matrixmanopt, absil12projectionretraction}. In our work, we consider the Euclidean Projection onto the Stiefel manifold given by the SVD. However, Pymanopt by default defines the retraction via the QR decomposition (although SVD-based retractions are also supported). In theory, this should yield similar convergence results in theory and practice.

We also consider the second-order trust-region method supported by Pymanopt~\cite{absiltrust}. We note that one contribution of our work is the extension of SSM, a state of the art method for large-scale trust-region subproblems to more general QCQPs. More generally, our generalization and application of SSM is motivated by its success on large scale trust-region subproblems (which our problem shares many characteristics with) - with remarkable empirical results and robust convergence guarantees, even for so-called ``degenerate problems''. SSM has many advantages over typical methods for Riemannian optimization (including first and second-order trust-region methods). To summarize, we claim that our proposed SSM method + Procrustes initialization, designed specifically for the problem we propose should outperform the more general techniques implemented in Pymanopt.

We show in Fig.~\ref{fig:foc} that the choice of subspaces play a critical role in the rate and quality of convergence of our method (compared to first-order methods). One may also ask how our method compares to traditional second-order methods (e.g. Riemannian Trust-region). In theory, SSM employs a special set of vectors to estimate the Hessian information to update the search direction via subspace minimization. As a result, the Hessian information estimated from SSM is usually better than the Hessian estimated from CG or BFGS methods typically used for trust-region type approaches.

Figure \ref{fig:knn} shows the accuracy of SSM at 5 labels per class as a function of the number of neighbors $K$ used in constructing the graph, showing that the algorithm is not significantly sensitive to this choice. 

%
%In Figure \ref{fig:labels_per_class}, we demonstrate the scaling behavior of our method. As the number of labels increases, our method is able to maintain high-quality predictions and consistently outperforms Laplace learning. 
%
In Figure \ref{fig:foc}, we demonstrate the convergence behavior of SSM and the projected gradient method discussed previously by plotting the norm of the first order condition (FOC): $||LX_tC - BC^{1/2}-X_t\Lambda_t||$. Note that while both methods are guaranteed to monotonically reduce the objective of \eqref{eq:rescaled_f} via line search, SSM rapidly converges to a critical point, while the projected gradient method fails to converge, even after 100 iterations.

\section{Graph-Based Active Learning}
\label{sec:activelearning}
In this section, we provide additional justification for the sampling score proposed in the main text. As mentioned in the main text, the component of score involving the eigenvector of $L_\mathcal{U}$ associated with the smallest eigenvalue is motivated primarily by previous work that investigates features encoded by the eigenvectors of the Laplacian of a graph with grounded vertices~\cite{cheng2019diffusiongeom}. These features specifically facilitate efficient methods to diversely sample the graph. Additionally, our score has connections to the graph signal processing literature~\cite{ajinkya2018distancesampling,anis215graphsampling} which aims to robustly recover a graph signal by sampling a sparse set of vertices. It has been demonstrated that one ideal sampling strategy that is robust to noise aims to maximize the smallest eigenvalue of the principal submatrix of the Laplacian, analogous to $L_\mathcal{U}$. Below, we demonstrate that our method, namely squaring the entries of $u$ and weighting by $\tilde{d}_i$, is directly related to one lower bound of the smallest eigenvalue of $L_\mathcal{U}$.

\subsubsection{Lower bound estimate for eigenvalues of $L_\mathcal{U}$}
Consider a grounded Laplacian $L_\mathcal{U}$ and the associated perturbation implied by labeling a vertex $E^i = \sum_{j \in \mathcal{U}}A_{ij} (E_{ij} + E_{ji})$, where $E_{ij}$ is an $n\times n$ matrix with $(L_\mathcal{U})_{ij}$ in the $ij$-th position (and, to be clear, $A_{ij}$ is a scalar). Let $u$ be one eigenvector of $L_\mathcal{U}$. Then, we have that the bound essentially follows from a proof of Weyl's inequality~\cite{horn13}.  If $G$ is connected or $|\mathcal{U}^c| > 0$, the eigenvectors of $L_\mathcal{U}$ form a basis for $\mathbb{R}^n$.
Let $v$ be a unit eigenvector of $L_\mathcal{U} - E^i$ with eigenvector decomposition (where $u^{(j)}$ is the eigenvector associated with the $j$-th eigenvalue of $L_\mathcal{U}$ ).
$$
v = \sum_{j=1}^n t_j u^{(j)}
$$
for some coefficients $t_j$ s.t. $\sum_j t_j^2 = 1$. Then the eigenvalue $\lambda '$ of $L_\mathcal{U} - E^i$ is
\begin{equation}
\lambda' = v^\top (L_\mathcal{U} - E^i)v = \sum_{j=1}^n t_j^2 (\lambda_j - \langle u^{(j)}, E^i u^{(j)} \rangle) \geq \min_{j=1,\ldots,n}\{\lambda_j - \langle u^{(j)}, E^i u^{(j)} \rangle\}
\end{equation}
Thus, the maximum perturbation of the smallest eigenvalue of $L_\mathcal{U} - E^i$ is bounded below by the largest eigenvalue of $E^i$ (recall that $E^i$ has nonzero entries associated with the $i$-th column and $i$-th row of $L_\mathcal{U}$). Hence, to increase the eigenvalue of $L_\mathcal{U}$, a greedy selection implies the choice of $i$ that maximizes $-\langle u^{(j)}, E^i u^{(j)} \rangle= 2u^{(j)}_i \sum_{k \in \mathcal{U}} A_{ij} u^{(j)}_k$.

Note that when the spectral gap of $L_\mathcal{U}$ is large, $j$ need not be taken over $[n]$. More concretely, suppose $\lambda_{k' + 1} - \lambda_1 > \epsilon$, where $\epsilon$ is the largest eigenvalue of $\{E^i\:\: : \:\: i=1,\ldots, n\}$. Note that $\lambda' \geq \lambda$. Then,
\begin{equation}
\lambda' \geq \min \{\min_{j=1,\ldots,k'} \{ \lambda_j -  \langle u^{(j)}, E^i u^{(j)} \rangle \}, \lambda_{k' + 1} - \epsilon\} \geq \min_{j=1,\ldots,k'} \{\lambda_j - \langle u^{(j)}, E^i u^{(j)} \rangle\}
\end{equation}
We highlight that the spectral gap of graph Laplacians of graphs constructed on data, particularly KNN graphs, exhibit fast growth of the eigenvalues~\cite{ulriketutorial2007, lafondatafusion2006} and large spectral gaps. On such graphs, the low-frequency eigenvectors (eigenvectors corresponding to the smallest eigenvalues of the Laplacian) are ``smooth'' over the graph and the score presented in the main text is a good proxy for the above bound, i.e.
$2u^{(j)}_i \sum_{k \in \mathcal{U}} A_{ij} u^{(j)}_k \approx 2\tilde{d}_{i}(u_i)^2$. As we show below, using the ranking implied by \emph{just} $u_i$ corresponds to a diversity selection strategy that iteratively selects vertices that are far from the set of labeled nodes. Intuitively, weighting this measure by $\tilde{d}_i$ encourages selection of vertices that are \emph{well connected}. Experimentally, as shown in the main text, this also has the effect of improving results.

%
\iffalse
\begin{proposition}[Entries of the smallest eigenvector]
%For simplicity, let $\mathcal{L}$ be a normalized laplacian. Then, the eigenvalues of $\mathcal{L}$ are bounded between $-1$ and $1$. 
Let $u$ be the eigenvector of $L_\mathcal{U}$ corresponding to its smallest eigenvalue. For each vertex $v_i \in \mathcal{V} \setminus \mathcal{U}$, let $a_{v_i} = \frac{\sum_{v_j \in \{N_i \setminus u\}}u_j}{|\{N_i \setminus \mathcal{U}\}|}$. For any vertex $v_a$ such that $v_a \not \in N_s$ for any $s \in \mathcal{U}$ and $v_b$ such that $v_b \in N_s$ for some $s \in \mathcal{U}$, $a_{v_a} \geq u_i$ and $a_{v_b} \leq u_i$.
\end{proposition}

We have that the $ith$ entry of the eigenvectors of $L_\mathcal{U}$ are characterized by the system 
$$
d_i u_i - \sum_{v_j \in N_j \setminus \mathcal{U}}A_{ij}u_j = \lambda u_i.
$$
Note that
\begin{align}
\frac{\sum_{v_j \in \{N_i \setminus \mathcal{U}\}}u_j}{d_i} < u_i &= \frac{\sum_{v_j \in \{N_i \setminus \mathcal{U}\}}u_j}{d_i - \lambda }  \leq \frac{\sum_{v_j \in \{N_i \setminus \mathcal{U}\}}u_j}{d_i - 1}
\end{align}

Since the left-hand-side of the inequality corresponds to $a_{v_a}$ and right-hand-side corresponds to $a_{v_b}$, we have the bound.
\fi

\subsection{Spectral active learning score}
For the purposes of this section, we will consider a slightly different scoring function than the one presented in the main text. Let $s(v_i) = |u_i|$, where $u_i$ is the $i$-th component of the eigenvector of $L_\mathcal{U}$ corresponding to the smallest eigenvalue of $L_\mathcal{U}$. Note that 
%(1.) $0 < \lambda \leq 1$ due to interlacing and (2.) 
when the graph is connected, from the Perron-Frobenius theorem~\cite{1miekkalagraphprop93, horn13}, the eigenvector associated with the smallest eigenvalue of $L_\mathcal{U}$ can be chosen to be elementwise nonnegative.
\begin{proposition}
Let $N_i$ denote the neighborhood of vertex $i$. Consider the score at vertex $v_a$, $s(v_a) = |u_i|$. For any connected pair of vertices $v_a$ and $v_b$ such that $v_a \not \in N_k$, $v_b \in N_k$ for any $k \in \mathcal{U}^c$, there is a path from $v_a$ to $v_b$ such that the sequence of entries $(s(v_a),\ldots, s(v_c), \ldots s(v_b))$ is nonincreasing.
\end{proposition} 
\noindent \emph{Proof.} We will consider a vertex $v_i$ and its score $s(v_i)$ when its neighborhood does not contain a labeled vertex and its score $s'(v_i)$ when its neighborhood does contain a labeled vertex, $v_\ell$. First, note that the $ith$ entry of the eigenvectors of $L_\mathcal{U}$ are characterized by the system 
$$
d_i u_i - \sum_{v_j \in \mathcal{U}}A_{ij}u_j = \lambda u_i.
$$
Then, write $u_i = \frac{\sum_{v_j \in \mathcal{U}}A_{ij}u_j}{d_i - \lambda }$ and consider labeleing a single neighbor $v_\ell$ in the neighborhood of $v_i$:
%\begin{align}
%\frac{\sum_{v_j \in \{N_i \setminus \mathcal{U}\}}u_j}{d_i} < u_i &= \frac{\sum_{v_j \in \{N_i \setminus \mathcal{U}\}}u_j}{d_i - \lambda }  \leq \frac{\sum_{v_j \in \{N_i \setminus \mathcal{U}\}}u_j}{d_i - 1}
%\end{align}
%\begin{align}
%s(v_i) = \tilde{d_i}|u_i| = d_i\left| \frac{\sum_{j \in \mathcal{U}}A_{ij}u_j}{d_i - \lambda} \right|  &=  d_i\frac{\sum_{j \in \mathcal{U}}A_{ij}|u_j|}{|d_i - \lambda|} \\
%&\geq  d_i\frac{\sum_{j \in \mathcal{U}}A_{ij}|u_j|- |u_\ell|}{|d_i - \lambda|} = d_i\left | \frac{\sum_{j \in \mathcal{U}\setminus \{u_\ell\}}A_{ij}u_j}{d_i - \lambda} \right|\\
%&\geq (d_i-1)\left| \frac{\sum_{j \in \mathcal{U}\setminus \{u_\ell\}}A_{ij}u_j}{d_i - \lambda} \right| = s'(v_i)
%\end{align}
\begin{align}
s(v_i) = |u_i| = \left| \frac{\sum_{j \in \mathcal{U}}A_{ij}u_j}{d_i - \lambda} \right|  &=  \frac{\sum_{j \in \mathcal{U}}A_{ij}|u_j|}{|d_i - \lambda|} \\
&\geq  \frac{\sum_{j \in \mathcal{U}}A_{ij}|u_j|- |u_\ell|}{|d_i - \lambda|} = \left | \frac{\sum_{j \in \mathcal{U}\setminus \{u_\ell\}}A_{ij}u_j}{d_i - \lambda} \right|\\
& = s'(v_i)
\end{align}
Naturally, the implication is that the score of a vertex decreases as its neighbors are labeled. Furthermore we have that
%\begin{align}
%s(v_i) = \tilde{d_i}|u_i| &= \tilde{d_i}\left| \frac{\sum_{j \in \mathcal{U}}A_{ij}u_j}{d_i - \lambda} \right| \geq \frac{1}{d_i}|\sum_{j \in \mathcal{U}}\tilde{d_j}A_{ij}u_j| = \frac{1}{d_i}\sum_{j\in \mathcal{U}}A_{ij}s(v_j)
%\end{align}
\begin{align}
s(v_i) = |u_i| &= \left| \frac{\sum_{j \in \mathcal{U}}A_{ij}u_j}{d_i - \lambda} \right| \geq \frac{1}{d_i}\left|\sum_{j \in \mathcal{U}}A_{ij}u_j\right| = \frac{1}{d_i}\sum_{j\in \mathcal{U}}A_{ij}s(v_j)
\end{align}
Thus, the score of a vertex $v_i$ is greater than the average score of its neighbors, and therefore, there must be a neighbor of $v_i$ with score less than $s(v_i)$. 
%Note that the bound may not hold unless $|\mathcal{N}(v_i)|\tilde{d_i} \geq \sum_{j\in \mathcal{U}}\tilde{d}_j$
%
Since each vertex has a neighbor with smaller score, starting from any vertex there is a path consisting of vertices that have decreasing scores that must finish at a vertex with neighbor in $\mathcal{U}^c$. \hfill \qedsymbol

Again, we emphasize that this is not necessarily true when $|u_i|$ is weighted by the degree $\tilde{d_i}$. Including this weight is intuitively motivated by the principle of connectnedness. In other words, our score selects vertices \emph{that are both distant from the set of labeled vertices, \textbf{and} well-connected}.

%Since the left-hand-side of the inequality corresponds to $a_{v_a}$ and right-hand-side corresponds to $a_{v_b}$, we have the bound.

%specifically the eigenvectors $U$, can be accomplished using an iterative Rayleigh-quotient minimization based algorithm. Specifically, the locally-optimal block preconditioned conjugate gradient (LOBPCG) method~\cite{lobpcg} is one state of the art approach. Typically, these methods necessitate matrix-vector products $L_\mathcal{U} x$ and the graphs encountered in canonical learning applications are sparse, leading to efficient implementations of $L_\mathcal{U} x$ in time linear in $|E|$, $O(|E|)$ the number of nonzero entries of $L_\mathcal{U}$. The complexity of each eigen-pair computation for $L_\mathcal{U}$ is then $O(d|E|t)$, where $t$ is a small constant equal to the average number of iterations required for the LOBPCG algorithm (note $t$ depends on the spectral properties of $L_\mathcal{U}$ and is independent of its size, i.e. $|V|$). In addition to computing the eigenpairs, selecting vertices iteratively to label requires a single pass through each vertex score, a linear-time operation. 


%
%$$
%u^\top \Delta L_\mathcal{U} u + u^\top \Delta L_\mathcal{U} \Delta u = u^\top \Delta \lambda u + u^\top \Delta \lambda \Delta u,\implies 
%\Delta \lambda = \frac{u^\top \Delta L_\mathcal{U} \hat{u}}{u^\top \hat{u}} = \frac{u_i\hat{u}_j + u_j \hat{u_i}}{u^\top \hat{u}}
%$$
%

\section{Convergence of SSM and Additional Computational Results}
\label{sec:ssmconvergence}
% bertsekas99nonlinprog, absil07matrixmanopt, luenberger15linnonlinprog8, absil12projectionretraction, conn00trust, sorensen82newtontrust
\subsection{Preliminaries}
\begin{equation}\label{eq:rescaled_f_apdx}
\begin{aligned}
\min_{X :X\in \textrm{St}(n,k)} \langle X, L X C \rangle - \langle X, B C^{1/2} \rangle
\end{aligned}
\end{equation}
Quadratic minimization over the Stiefel manifold is a generalization of the well-known nonconvex quadratic over the unit ball or sphere. These problems often arise in trust region methods \cite{sorensen82newtontrust, conn00trust}. Notably, there could exist many local solutions in \ref{eq:rescaled_f_apdx}. We will demonstrate convergence to critical points of two iterative methods: a gradient projection method and the Sequential Subspace Method proposed in this work. Furthermore, when the subspaces component to the SSM algorithm contain the span of the first $k$ nontrivial eigenvectors of $L$, we show that the quality of the stationary point is characterized by the eigenvalues of the Lagranage multipliers $\Lambda$.

First denote the the eigenvector decomposition of $L$ be given by
$$
L = [v_1, v_2, \ldots, v_n]\text{diag}(d_1, \ldots, d_n)[v_1, v_2, \ldots, v_n].T
$$

To summarize, we will show the following:
\begin{itemize}
    \item We propose a gradient projection method to solve \ref{eq:rescaled_f_apdx}. We prove convergence with the Armijo rule in Prop.~\ref{prop:pgd_convergence}.
    \item We analyze the proposed iterative method in the framework of SSM, constructing a sequence of subspaces to reach one approximation of local solutions, where the subspace consists of columns of $X_t$, $LX_tC-BC^{1/2}$ and eigenvectors associated with $d_i$, $i=1,\ldots,k$. Each sub-problem can be solved by the aforementioned gradient projection method. We demonstrate global convergence to high-quality critical points. Theoretically, when $C=I$ and the multiplicity of the first nontrivial eigenvalue is greater than or equal to $k$, a local solution is actually a global solution. However, we leave this analysis as future work.
\end{itemize}
First, we review some known results in the spherical case, i.e., $\text{St}(n, 1)$. Next, we derive convergence of a projected gradient method to solutions satisfying the first order condition~\eqref{eq:rescaled_f_foc}. Finally, Theorem 1 states the convergence of SSM to a high-quality local solution is guaranteed.

\subsubsection{Notation}

We assume $k$ is a positive integer (much) less than $n$. Let $K$ denote the set $\{1, 2,\ldots , k\}$. Let $I_{n,k}$ denote the sub matrix of the identity matrix $I_n$, consisting of the first $k$ columns. Let $O_k$ be the orthogonal group, i.e., $Q \in O_k$ if and only if $Q \in \mathbb{R}_{k,k}$ and $Q^\top Q = I_k$.

\subsection{Preliminary results in the spherical case}
\eqref{eq:rescaled_f_apdx} is one natural generalization of the constrained problem \cite{Hager2001MinimizingAQ,Hager2005GlobalSSM}
\begin{equation}\label{eq:hager}
\min_x \{x^\top A x - 2\langle x, b\rangle: ||x|| = 1, x\in \mathbb{R}^n\}
\end{equation}
This problem is related to the trust region subproblem:
\begin{equation}\label{eq:trust}
\min_x \{x^\top A x - 2\langle x, b\rangle: ||x|| \leq 1, x\in \mathbb{R}^n\}
\end{equation}
The following two propositions describe the global solution of \ref{eq:hager}. See \cite{sorensen82newtontrust}. The condition \ref{eq:trust_opt_condition} states that the global solution $x$ is the critical point associated with $\lambda$ bounded above by the smallest eigenvalue $d_1$ of $A$.
%
\begin{proposition}[\citet{Hager2005GlobalSSM}]
A vector $x \in \mathbb{R}^n$ is a global solution of \ref{eq:hager}, if and only if $||x|| = 1$, and
\begin{equation}\label{eq:trust_opt_condition}
A - \lambda I \succcurlyeq 0, \:\: (A - \lambda I)x = b
\end{equation}
holds for some $\lambda \in \mathbb{R}$
\label{prop:global_solution}
\end{proposition}
%
\begin{proposition}[\citet{Hager2001MinimizingAQ}]
Consider the eigenvector decomposition 
$$
A = [v_1, v_2, \ldots, v_n]\text{diag}(d_1, \ldots, d_n)[v_1, v_2, \ldots, v_n].T.
$$
Let $V_1$ be the matrix whose columns are eigenvectors of $L$ with eigenvalue $d_1$. Then, $x = Vc$ is a solution for a vector $c$ chosen in the following way:
\begin{itemize}
\item Degenerate case: suppose $V_1^\top b = 0$ and $c_{\perp}:= ||(A - d_1I)^{\dagger}b||\leq 1$
Then, $\lambda = d_1$ and $x = (1 - c_\perp^2)^{1/2}v_1 + (A - d_1 I)^{\dagger} b$
\item Nondegenerate case: $\lambda < d_1$ is chosen so that $x = (A - \lambda I)^{-1}b$ with $||x|| = 1$.
\end{itemize}
\label{prop:plp}
\end{proposition}
%
\begin{remark}[\citet{Hager2005GlobalSSM}]
Note that $||(A - \lambda I)^{-1}b||$ decreases monotonically with respect to $\lambda\leq d_1$. A proper value of $\lambda$ meets the condition $||x|| = 1$. A tighter bound on $\lambda$ can be estimated from 
$$
(d_1 - \lambda) ||V_1b||^2 \leq 1 = ||(A - \lambda I)^{-1}b||^2 \leq (d_1 - \lambda)^{-2}||b||^2
$$
With $||V_1 b|| > 0$, $\lambda$ lies in the interval $[d_1 - ||b||, d_1 - ||V_1 b||]$
\label{prop:plp}
\end{remark}
%
\subsection{Computational results}
In this section, we provide the precise computations involved in the derivation of \eqref{eq:rescaled_f} from \eqref{eq:supervised_lapeig}.
\subsubsection{Derivation of $B$ and $C$}

Given $\mathbf{1}^\top X = 0$ and $X^\top X = pI$, we have that $\mathbf{1}^\top X_\mathcal{U} = -r^\top$ and $X_\mathcal{U}^\top X_\mathcal{U} = pI - X_l^\top X_l = (p-\widetilde{p})I$, where $r = \mathbf{1}^\top X_l$.

Let $(\widetilde{X}_{\mathcal{U}})_i = (X_{\mathcal{U}})_i + \frac{1}{n}r$. We have the following:
\begin{enumerate}
\item $\mathbf{1}^\top \widetilde{X}_{\mathcal{U}} = 0$
\item $X_\mathcal{U}^\top X_\mathcal{U} = \widetilde{X}_{\mathcal{U}}^\top\widetilde{X}_{\mathcal{U}} + \frac{1}{n} r^\top r$
\end{enumerate}
Thus, $\widetilde{X}_{\mathcal{U}}^\top \widetilde{X}_{\mathcal{U}} = (p-\widetilde{p})I - \frac{1}{n} r^\top r$

Consider $\langle X_0, LX_0 \rangle =  X_\mathcal{U}^\top L_\mathcal{U} X_\mathcal{U} + 2X_\mathcal{U}^\top L_{\mathcal{U}l}X_l + X_l^\top L_l X_l$. Let 
$R = \frac{1}{n}\left[\begin{smallmatrix}
r^\top\\
\vdots \\
r^\top
\end{smallmatrix}\right] \in \mathbb{R}^{n\times k}$
We have that
\begin{flalign*}
\langle X_0, LX_0 \rangle &= \widetilde{X}_{\mathcal{U}}^\top L_\mathcal{U}\widetilde{X}_{u} - 2\widetilde{X}_{\mathcal{U}}^\top L_\mathcal{U}R \\
&+R\top L_\mathcal{U} R + 2\widetilde{X}_\mathcal{U}^\top L_{\mathcal{U}l}X_l - 2R^\top L_{\mathcal{U}l}X_l + X_l^\top L_l X_l \\
&= \widetilde{X}_\mathcal{U}^\top L_\mathcal{U} \widetilde{X}_\mathcal{U} + 2\widetilde{X}_\mathcal{U}^\top (-L_\mathcal{U} R + L_{\mathcal{U}l}X_l) \\
&+ R^\top L_\mathcal{U} R - 2R^\top L_{\mathcal{U}l}X_l + X_l^\top L_l X_l
\end{flalign*}

\subsubsection{Pseudo-inverse of $PL_\mathcal{U}P$, definiteness conditions of $X^\top B$, SQP Direction $Z$}

Several of the algorithms we describe necessitate computation of pseudoinverse-vector products of the perturbed Laplacian $PL_\mathcal{U}P$\textemdash i.e. $(PL_\mathcal{U}P)^{\dagger}u$. Here, we demonstrate that the computation of $(PL_\mathcal{U}P)^{\dagger}u$ is computationally comparable to computing a standard laplacian pseudoinverse-vector product, $L_\mathcal{U}^{\dagger}u$, for which there exist nearly linear-time solvers~\cite{spielmanteng}.
\begin{proposition}[Psudo-inverse of $PL_\mathcal{U}^{-1}P$]
Let $P = I - vv^\top$ for a unit vector $v$. Let $r_k = \{PL_\mathcal{U}^{-1}P\}^\dagger u_{k-1}$. Then, the projection of $r_k$ is
$$
Pr_k = \{PL_\mathcal{U}^{-1}P\}^\dagger u_{k-1} = (I - \frac{\bar{v}^\top v}{v^\top \bar{v}})L_\mathcal{U}^{-1}u_{k-1},\quad \bar{v} = L_\mathcal{U}^{-1}v
$$
\label{prop:plp}
\end{proposition}

\begin{proposition}[Definiteness conditions of $X^\top B$]
Assume $C = I$. Note the first term of $F$ satisfies the invariance $\text{tr}(X^\top LX) = \text{tr}(\widetilde{X}^\top L\widetilde{X})$, where $\widetilde{X} = XQ$ for any orthogonal $Q \in \mathbb{R}^{2\times2}$. $X$ is a local minimizer if $X^\top B\succcurlyeq 0$ and symmetric. 
%\label{rem:negdef}
\end{proposition}
\emph{Proof.} Note that by assumption, $X$ is feasible\textemdash i.e. $X^\top X = I$. Consider the substitution $X \to XQ$ for some orthogonal matrix $Q$. Since $C = I$, $F(XQ) = \langle XQ, LXQ \rangle - \langle Q, X^\top B \rangle$.

Fix $X$. Note that the first term satisfies the invariance $\langle X, LX \rangle = \langle XQ, LXQ \rangle$. For any orthogonal $Q \in \mathbb{R}^{k\times k}$. The optimal choice of $Q$ is determined by the second term. A standard result from matrix analysis yields its minimizer~\cite{horn13}. Let $X^\top B = UDV^\top$ be the SVD of $X^\top B$. Then, $Q = U_B V_B^\top$ and $\langle XQ, B\rangle = \langle Q, X^\top B \rangle = \langle I, D \rangle = tr(D) \geq 0$. \qedsymbol
%
\begin{proposition}[SQP Direction of the Lagrangian Eq.~\eqref{eq:rescaled_f_lagrangian}]
Assume $\Lambda$ symmetric. Let $P$ be a projection matrix and $\Lambda C^{-1} = U\text{diag}([\lambda_1, \ldots \lambda_k]) U^{-1}$ be the eigenvector decomposition of $\Lambda C^{-1}$. The solution to the newton direction $Z$ of $X$ via the linearization of the FOC is given by 
%
\begin{equation}
  Z = OU^\top
  %\label{eq:newton_direction}
\end{equation}
%
where each column of $O$, $o_j = (PLP - \lambda_j P)^\dagger BC^{-1}u_j$.
%\label{prop:newton}
\end{proposition}
\emph{Proof.} Recall the FOC and its associated linearization with respect to descent directions of $X, \Lambda$; $(Z, \Delta)$:
\begin{align*}
&(LZC - Z\Lambda) - X \Delta = E := BC^{1/2} - (LXC - X\Lambda) \\
&X^\top Z = 0
\end{align*}
Applying the projection $P^{\perp} = I - XX^\top$ eliminates the $X\Delta$ term:
$$
PLZ - Z\Lambda C^{-1} = PLPZ - ZU\text{diag}([\lambda_1, \ldots, \lambda_k])U^{-1} = PEC^{-1}
$$
Equivalently, 
$$
PLPZU - ZU\text{diag}([\lambda_1, \ldots, \lambda_k]) = PEC^{-1}U.
$$ 
Let $O = ZU = [o_1,\ldots, o_k]$ lie in the range of $P$. Then, 
$$
PLo_j - \lambda_j = PEC^{-1}u_j, \text{ so } o_j = (PLP - \lambda_j P)^\dagger EC^{-1}u_j.
$$ \qedsymbol
%
\iffalse
Note that $\lambda_j$ appears in the computation of the pseudo inverse of $P^\perp L P^\perp - \lambda_j P^\perp$. To ensure that $P^\perp L P^\perp - \lambda_j P^\perp$ is positive semi-definite, we introduce a \emph{safeguard} to adjust $\lambda_j$ manually. 
%
\begin{proposition}[Safeguard for $\lambda_j$]
$\lambda_j$ are chosen to be the eigenvalues of $\Lambda C^{-1}$. Let
$$
P_1^{\perp} = P^{\perp} + x
$$
\end{proposition}
We note that the safeugarding $\lambda_j$ introduces additional computational  our algorithm. In practice, we observe that safeugarding is not necessary\textemdash i.e. for all of our experiments, we forgo safeguarding to save computation. 
\fi

%\begin{proposition}[Effect of Laplacian normalization]
%Consider the rescaled problem...where $D$ is a strictly positive definite diagonal matrix. We claim that this is equivalent to solving the original problem (with no $D$ or $D = I$).
%\end{proposition}
%\emph{Proof. } Consider a 

\subsection{Convergence of the Projected Gradient Method (PGD)}
We first introduce a projected gradient-based method. With appropriate step size $\alpha > 0$, PGD produces iterates $X_t$, $t = 1, 2, \ldots$
$$
X_{t+1} = [X_t - \alpha g_t]_+
$$
Where $g_t$ is given by the gradient of the objective of \eqref{eq:rescaled_f_apdx}\textemdash i.e. $g_t = LX_tC - BC^{1/2}$ and $[X_t]_+$ is the projection onto the manifold
$$
\mathcal{M} := \{X : X \in St(n,k), X^\top B \geq 0\}
$$
We first describe the projection $X = [X_1]_+$ as a composition of two projections; i.e. $[X_1]_+ = [[X_1]_{St}]_\mathcal{B} \in \mathcal{M}$:
\begin{flalign}
& Z = [X_1]_{St} := \argmin_Z \{||X_1 - Z||_F : Z \in St(m,r)\} \label{eq:stproj} \\
& X = [Z]_\mathcal{B}:= ZQ,\:\:Q=\argmin_Q \{||Z - BQ^\top||_F : Q \in O_k\} \label{eq:Bproj}
\end{flalign}
In other words, $Z \in St(n,r)$ and $Q \in O_k$ are chosen to minimize the sum
$$
||X_1 - Z||_F^2 + ||Z - BQ^\top||_F^2 = ||X_1Q - ZQ||^2_F + ||ZQ - B||_F^2
$$
Take the SVD of $X_1$, i.e. $X_1 = U_XD_XV_X^\top$. Then, the solution to \eqref{eq:stproj} is given by $Z = U_XV_X^\top$. Likewise, $X=ZQ$ for some orthogonal matrix $Q$ chosen to maximize $\langle X, B \rangle = X^\top B$. 

\begin{proposition}[Projection onto $\mathcal{B}$]\label{prop:projection}
Consider the solution to the following projection:
\begin{equation}\label{eq:proj_apdx}
[X_1]_+ = \argmin_{X\in St(n,k)}\{\min_Q ||X - X_1Q||_F^2 : X^\top B \geq 0, Q \in O_k\}
\end{equation}
Suppose the singular values of $X_1$ and $B$ are positive. Then, the minimizer $X$ is uniquely determined by 
$$
X = [X_1]_+ = U_1 U_2 V_2^\top
$$
where $U_1, V_1, V_2$ are determined from the two SVDs,
$$
U_1 \Sigma_1 V_1^\top = X_1, \:\: U_2\Sigma_2V_2^\top = U_1^\top B
$$
\end{proposition}
\emph{Proof.} The minimizer $X$ in \eqref{eq:proj_apdx} is the maximizer of $\max_X \langle X, X_1 Q\rangle$. Note that
$$
\langle X, X_1 Q\rangle = \langle X, U_1 \Sigma_1 V_1^\top Q \rangle = \langle U_1^\top X Q^\top V_1, \Sigma_1 \rangle \leq tr(\Sigma_1)
$$
Note two observations: (1) that $U_1^\top X Q^\top V_1$ lies in $O_k$, and (2) that equality holds if and only if $U_1^\top X Q^\top V_1 = I_k$ for some $XQ^\top V_1 \in \text{St}(n, k)$, i.e. $XQ^\top V_1 = U_1$, and thus,
$$
X = U_1 V_1^\top Q.
$$
Furthermore, the condition $X^\top B$ is symmetric and positive definite implies a choice of $Q$ that fulfills 
$$
X^\top B = Q^\top V_1 U_2 \Sigma_2 V_2^\top, \:\: i.e., V^\top Q = V_2 U_2^\top
$$
Finally, note that since the singular values $\Sigma_1, \Sigma_2$ are distinct and positive, $U_1$ and $V_1$ are uniquely determined up to column-sign $Q_1 = \text{diag} (\pm 1, \ldots \pm 1)$. Likewise, $U_2$ and $V_2$ are uniquely determined up to $Q_2 = \text{diag} (\pm 1, \ldots \pm 1)$. Hence,
$$
X = U_1 Q_1 Q_2^\top U_2 Q_2 Q_2^\top V_2^\top = U_1 U_2 V_2^\top
$$
is unique. \qedsymbol

\begin{remark}\label{rem:differential}
Consider the function $h(X) = [X]_{\text{St}}$ defined on $\mathbb{R}^{n\times k}$ and $X\in St(n,k)$. The differential $\mathbb{D}h$ at $X$ is the linear map given by
$$
\mathbb{D}h(X)[T] - \lim_{\alpha \to 0}\alpha^{-1}(h(X + \alpha T)-h(X)) = (I - XX^\top)T + (-1/2)X(T^\top X - X^\top T)
$$
for each $T\in \mathbb{R}^{n\times k}$. When $X \in \mathcal{M}$ and $T = -(LXC - BC^{1/2})$, then
$$
\langle T, \mathbb{D}h(X)[T] \rangle = ||(I- XX^\top)T||_F^2.
$$
\end{remark}

\begin{proposition}\label{prop:pgd_convergence}
Let $d_t = -(LX_tC - BC^{1/2})$. Let $\{X_t\}$ be a sequence generated by the gradient projection method
$$
X_{t+1} = [x_t + \alpha_t d_t]_+
$$
where $\alpha_t$ is chosen according the Armijo rule. Then, every limit point of $\{X_t\}$ is a stationary point.
\end{proposition}
\emph{Proof.} The proof is motivated by the proof by contradiction of Prop. 1.2.1 in \citet{bertsekas99nonlinprog}.

Let $\mathcal{G}(X) = (I - X^\top X)(AXC - BC^{1/2})$ be the projected gradient of the objective of \ref{eq:rescaled_f_apdx}, $F$ at $X$. We define $\alpha$ given by the Armijo rule\textemdash i.e. let $s > 0$, $\sigma \in (0,1)$ and $\beta \in (0,1)$. $\alpha_t = \beta^{m_t}s$, where $m_t$ is the first nonnegative integer $m$ for which
$$
F(X_t) - F([X_t + \beta^msd_t]_+)\geq -\sigma \beta_t s\langle \mathcal{G}(X_t), d_t \rangle
$$
Suppose $\hat{X}\in \mathcal{M}$ is a limit point of $\{X_t\}$ with $||\mathcal{G}(\hat{X}|| > 0$. By definition, $\{F(X_t)\}$  is monotonically nonincreasing to $F(\hat{X})$., i.e. $F(X_t) - f(X_{t-1}) \to 0$. By definition, since the $\alpha_t$, the step sizes are generated via the Armijo rule, $a_t$ satisfies
\begin{equation}\label{eq:armijo}
\begin{aligned}
F(X_t) - F(x_{t+1}) &\geq F(X_t) - F([X_t + \alpha_t d_t]_+) \\
&\geq -\sigma \langle \mathcal{G}(X_t), d_t \rangle = \sigma \alpha_t ||\mathcal{G}(X_t)||_F^2
\end{aligned}
\end{equation}
Let $\{X_t\}_{\mathcal{T}}$ be a subsequence converging to $\hat{X}\in \mathcal{M}$ Since 
$$
\lim_{t \to \infty} \sup -\langle \mathcal{G}(X_t), d_t \rangle = ||\mathcal{G}(\hat{X})||^2 > 0,
$$
\eqref{eq:armijo} implies $\{\alpha_t\}_{\mathcal{T}}\to 0$. From Armijo's rule, for some $t'\geq 0$, the inequality
\begin{equation}\label{eq:armijo2}
F(X_t) - F([X_t + \alpha_t \beta^{-1}d_t]_+)< -\sigma \alpha_t \beta^{-1} \langle \mathcal{G}(X_t), d_t \rangle
\end{equation}
holds for all $t \geq t'$. By taking a subsequence $\{d_t\}_{\mathcal{T}'}$ of  $\{d_t\}_{\mathcal{T}}$ such that $\{d_t\}_{\mathcal{T}'} \to d'$ and $X_t \to X'$, applying the mean value theorem to the left hand side of \eqref{eq:armijo2}, we have that
\begin{flalign*}
&-\langle L([X_t + \alpha_t' d_t]_+C) - B, \mathbb{D}([X_t + \alpha_t' d_t]_+)[d_t] \rangle \\
&=(\alpha_t \beta^{-1})^{-1}(F(X_t)) - F([X_t + \alpha_t \beta^{-1}d_t]_+) \\
&< -\sigma \langle \mathcal{G}(X_t), d_t\rangle
\end{flalign*}
for some $\alpha_t' \in [0, \alpha_t\beta^{-1}]$. Taking the limit as $k\to \infty$, we have that $\alpha_t'\to 0$ and $\mathbb{D}([X_t + \alpha_t' d_t]_+)[d_t] \to \mathcal{G}(X')$, which implies 
$$
-\langle \mathcal{G}(X'), d' \rangle \leq -\sigma \langle \mathcal{G}(X'), d' \rangle, \:\: \text{i.e. } -(1-\sigma)\langle \mathcal{G}(X'), d' \rangle \leq 0
$$
Since $\sigma < 1$, it follows that 
$$
-\langle \mathcal{G}(X'), d' \rangle = ||\mathcal{G}(X')||_F^2 \leq 0
$$
which contradicts the non-stationarity of $X'$. Hence, the limit point $\hat{X}$ is a stationary point. \qedsymbol

\subsection{Convergence of SSM}
The proof follows from the associated result for the Projected Gradient Method, Prop.~\ref{prop:pgd_convergence}\textemdash i.e. applying the Projected Gradient Method with step sizes chosen according to the Armijo rule ensures that any limit point $X_*$ is a stationary point, when $d_t = -(LX_tC - BC^{1/2}) \in S_t$. Let $V_t$ be an isometry, consisting of vectors in $S_t$ computed via a QR-factorization. Let $L_t := V^\top_t L V_t$ and $B_t = V_t^\top B$. Then, $F(\widetilde{X}; L_t, B_t)$ be the corresponding objective in $S_t$. SSM computes $X_{t+1} = V_t\widetilde{X}$, where
$$
\widetilde{X} := \argmin_{\widetilde{X}} F(\widetilde{X}; L_t, B_t)
$$
Note that the sequence $\{X_1,\ldots, X_t, \ldots\}$, with $X_{t+1}\in V_t$ monotonically reduces $F$ with respect to $t$:
\begin{flalign*}
F(\widetilde{X}; L_t, B_t) &= \frac{1}{2}\langle X_{t+1}, LX_{t+1}C - 2BC^{1/2} \rangle \\
&\leq \min_{\widetilde{X}}\{\frac{1}{2}\langle V_t\widetilde{X}, LV_t\widetilde{X}C - 2BC^{1/2} \rangle = \frac{1}{2}\langle \widetilde{X}, L_t\widetilde{X}C - 2B_tC^{1/2} \rangle = F(\widetilde{X}; L_t, B_tC^{1/2})\} \\
&\leq \frac{1}{2}\langle X_t, LX_tC - 2BC^{1/2} \rangle = F(X_t; L, B)
\end{flalign*}
For each $t$, since the columns of $X_t$ and $LX_tC - BC^{1/2}$ lie in $S_t$, the iterations of the gradient projection method with Armijo rule lie in $S_t$, and the sequence with decreasing objective reaches a stationary point $\widetilde{X}$, it is ensured that the first order condition
$$
AX_*C - BC^{1/2} = X_*\Lambda_*
$$
holds for some matrix $\Lambda_* \in \mathbb{R}^{k\times k}$, given by
$$
\Lambda_* = X_*^\top (LX_*C - BC^{1/2}) = \lim_t X_t^\top(LX_kC - BC^{1/2})
$$
In the case $C = I$, the following states that the inclusion of $[v_1, \ldots, v_k]$ in $S_t$ improves the quality of the stationary point $X_*$, characterized by the eigenvalues of $\Lambda$.

\begin{proposition}[Convergence of SSM]\label{prop:ssm_convergence}
Assume $C = I$. Let $X_* := [x_1,\ldots,x_k]$ be a stationary point generated from SSM. Then,
$$
LX_* - X_*\Lambda_* = B.
$$
Let $\lambda_1,\ldots,\lambda_k$ be the eigenvalues of $\Lambda_*$ and let the eigenvalues of $L$ be $d_1 \leq d_2 \leq \ldots \leq d_n$. Then, $\max\{\lambda_1,\ldots,\lambda_k\} \leq d_k$. 
\end{proposition}

\emph{Proof. } Let $X_t = [x_{1,t}, \ldots, x_{k,t}]$ be a global minimizer in $V_{t-1}$. let $Y_t := [y_{1,t}, \ldots, y_{k,t}] = V_{t-1}^\top [x_{1, t}, \ldots, x_{k,t}]$. Then,
$$
L_{t-1}Y_t - B_{t-1} = Y_t \Lambda_t
$$
holds for some $\Lambda_k$ with eigenvalues $[\lambda_{1,t}, \ldots, \lambda_{k,t}]$. In addition, since $Y_tB_{t-1} = X_tB$, then $X_tB$ is positive semidefinite and symmetric. As $t \to \infty$, $X_*^\top B$ is also positive semidefinite and symmetric. Additionally, let
$$
P_j^{\perp, (t)} = I - \sum_{i \in \mathcal{R} - {j}} y_{i,t}y_{i,t}^\top.
$$
The second order condition implies
$$
P_j^{\perp, (t)}LP_j^{\perp, (t)} - \lambda_{j,t}P_j^{\perp, (t)} \succeq	0.
$$
Consider the optimality of $x_{1,t}$. Let $\phi_{1,t}$ by a unit vector orthogonal to $[x_{2,t},\ldots, x_{k,t}]$ in $span\{v_1,\ldots,v_k\}$. Then $P_j^{\perp, (t)}V_{t-1}^\top \phi_{1,t} = V_{t-1}^\top\phi_{1,t}$ holds and the second order condition yields
\begin{flalign*}
0&\leq \langle V_{t-1}^\top\phi_{1,t}, (P_j^{\perp, (t)}LP_{j,t}^{\perp} - \lambda_{j,t}P_{j,t}^{\perp})V_{t-1}^\top \phi_{1,t} \rangle \\
&= \langle \phi_{1,t}, (L - \lambda_{1,t}I)\phi_{1,t}\rangle\\
&\leq (\min_i d_i - \lambda_{1,t})||\phi_{1,t}||^2,
\end{flalign*}
Which implies $\lambda_{1,t} \leq \min_i d_i$. As $t \to \infty$, a subsequence of $\{x_{1,t}, \ldots, x_{k,t} : t \}$ converges to $[x_1,\ldots, x_k]\in \mathcal{M}$ and $\lambda_{1,t}$ converges to $\lambda_1$ Hence, $\lambda_1 \leq \min_i d_i$. Likewise, $\lambda_j \leq \min_i d_i$ by the optimality of $x_{j,t}$ for $j = 2,\ldots, k$. \qedsymbol

The following is the result of \Cref{prop:ssm_convergence}.
%\input{statements/ssm_convergence.tex}
\ssm*

\textbf{On convergence to globally optimal solutions}

We briefly and informally discuss the necessary conditions for \emph{global optimality} of \eqref{eq:rescaled_f}, under the assumption that $C= I$. For simplicity, take $k=2$. And denot $\lambda_1, \lambda_2$ the eigenvalues of $\Lambda$. We can prove that for any local minimizer $X$, if the associated eigenvalues $\lambda_1,\lambda_2$ are both less than $d_1$, the smallest nonzero eigenvalue of $L$, that $X$ is a global minimizer. As we have shown, with proper initialization, our method recovers a local minimizer $X$ such that $\lambda_1, \lambda_2$ are both less than $d_2$. There are several potential avenues to prove that any local minimizer is also a global minimizer. For example we could impose an eigenvector-preserving transformation to $L$ or restrict our analysis to graphs such that $\lambda_i = \lambda_k$ where $\lambda_i \geq 0$. 

An alternative method is to ensure a non-degenerate condition on $B$ as in canonical trust-region methods. Briefly, let $v_1, \ldots, v_k$ be the eigenvectors of $L$ corresponding to $k$ smallest nonzero eigenvalues $d_1 \leq \ldots \leq d_k$. At a high level, we need to ensure that the columns of $B$ are not nearly orthogonal to $v_1, \ldots, v_r$

\begin{proposition}
Let $V = [v_1, v_2]\in \mathbb{R}^{n \times 2}$ be the eigenvectors of $L$ corresponding to the smallest two nonzero eigenvalues $d_1 \leq d_2$. Let $X$ be a local solution satisfying the first order condition 
$$
AX = X\Lambda + B
$$
and second order condition $\lambda_1, \lambda_2 \leq d_2$. Let $s_1$ be the smallest singular value of $V^\top B$. Suppose
$$
s_1 > d_2 - d_1
$$
Then, the eigenvalues $\lambda_1, \lambda_2$ of the Lagrangian multipliers $\Lambda$ are less than $d_1$ and $X$ is a global minimizer.
\end{proposition}
\emph{Proof. } Recall that the second order condition is 
$$
\lambda_j \leq d_2 \text{ for } j = 1,2.
$$
Consider the first order condition $LX = X\Lambda + B$. Taking an inner product with $v_2$ and $v_1$ yields
\begin{flalign*}
&d_2 v_2^\top X = v_2^\top LX = (v_2^\top X)\Lambda + v_2^\top B, \\
&d_1 v_1^\top X = v_1^\top LX = (v_1^\top X)\Lambda + v_1^\top B.
\end{flalign*}
Let $u_1$ and $u_2$ be eigenvectors of $\Lambda$ associated with eigenvalues $\lambda_1, \lambda_2$. For $j=1,2$, taking the product with $u_j$ on the r.h.s yields
$$
(d_2 - \lambda_j)v_2^\top Xu_j = v_2^\top Bu_j,\:\: (d_1 - \lambda_j)v_1^\top Xu_j = v_1^\top Bu_j 
$$
Since $||V|| = 1 = ||X||$, then $||V^\top X u_j||\leq ||Xu_j|| \leq 1$. Thus,
$$
|d_2 - d_1| < s_1 \leq ||V^\top B u_j|| \leq \min(|d_2 - \lambda_j|,|d_1 - \lambda_j|)||V^\top X u_j|| \leq \min(|d_2 - \lambda_j|,|d_1 - \lambda_j|)
$$
which implies $\lambda_j < d_1$.

%While the spectral gap (the difference between the smallest two eigenvalues) of the graph Laplacian has been intensely studied, there is sparse work about the multiplicity of second eigenvalue. One result is given by \cite{}, who characterize graphs with multiplicity of $\lambda_2$ greater than or equal to $k$ with degree-$d$ or bounded degree-$d$ graphs.

\section{Limitations and Societal Impact}
\label{sec:limitations}
Here, we list several limitations and briefly touch upon the broader societal impact of our method.
\begin{itemize}
\item Optimization variance: Our methods exhibit slightly larger variance predictions compared to Poisson learning. However, when our method is augmented with the KL refinement scheme, we see a significant decrease in the variance of predictions. In future work we intend to explore (1.) why SSM introduces variance in the solution and (2.) why cut-based refinement seems to remedy this issue.

\item Underlying graph structure: Much of this work relies on the structure of the underlying graph. In this work, we did not explore variations on the graph structure and setting the graph weights, instead opting for a relatively simple approach via neural networks to generate features for each node.

%\item Active learning: One extension that we did not explore for the sake of brevity was leveraging our decomposition and reliance on the Eigenvectors of the Laplacian to deduce samples that would be effective in helping the predictor perform well.
\end{itemize}

We have introduced a new method for graph learning that improves on the state of the art across multiple label-rate regimes. The development of such methods has positive and negative ramifications for civil liberties and human rights. While the positive ramifications are relatively clear- models which require less data are cheaper to train and are generally ``lower-impact''\textemdash the negative consequences are not immediately obvious. The above question is explored in greater detail in the content of semi-supervised graph learning in Fairness in graph-based semi-supervised learning, \citet{zhang2023fairness}. The principal claim made by \citet{zhang2023fairness} is that when quantities of unlabeled data are provided, label propagation may be modified to improve fairness. Interestingly, there seems to be an intimate relationship between methods designed to promote fairness and the cut-based MBO scheme proposed in Calder \cite{calder20poisson}.
